# Supplementary material for: What should I document? A preliminary systematic mapping study into API documentation knowledge
Source: arXiv:1907.13260 source file (2019-07-30)
Supplement: Supplementary file 1 [file primarysources.tex]

\documentclass[10pt,conference]{article}

% Useful packages included in extended preamble
\usepackage{import}
\import{../preamble/}{extended.tex}

\begin{document}

\nocite{Robillard:2009uk,Robillard:2011uv,Ko:2011fb,Nykaza:2002td,Watson:2013fx,Jeong:2009tu,Aghajani:2019bo,Haselbock:2018jd,Inzunza:2018dn,Meng:2017cx,Geiger:2018fv,Head:2018baa,Aversano:2017ic,Robillard:hk,Watson:2012uy,Maalej:2013uu,Parnas:2007fb,Bottomley:2005fs,Taulavuori:2004el,Kotula:1998wp,McLellan:1998vu}		
\bibliography{../papers}

\end{document}
